# Supplementary material for: Slowest kinetic modes revealed by metabasin renormalization
Source: arXiv:1802.06558 source file (2018-02-19)
Supplement: Supplementary file 1 [file SupplementalMaterial.pdf]

# Supplemental Material: Slowest kinetic modes revealed by metabasin renormalization

Teruaki Okushima, Tomoaki Niiyama, Kensuke S. Ikeda, Yasushi Shimizu

In this Supplemental Material, we will show that the renormalization procedure developed in the paper can be applicable to the discrete-time kinetic equations, also known as (discrete-time) Markov state models [1], with small modifications.

Suppose that the kinetic state is described by the distribution of probability, $p_i$, for $i = 1, 2, \dots, n$, where $n$ denotes the number of states, the kinetic equations are given by

$$p_i(t+1) = \sum_{j=1}^{n} t_{ij} p_j(t) + p_i(t)\Big(1 - \sum_{j=1}^{n} t_{ji}\Big) \quad \text{for } i = 1, 2, \dots, n, \tag{1}$$

where $p_i(t)$ is the probability distribution of the system state $i$ at discrete times $t = 0, 1, 2, \dots$, and $t_{ij}$ is the transition probability from state $j$ to state $i$ for $j \neq i$, otherwise $t_{ii} = 0$. With the transition *probability* matrix $T$ defined by $(T)_{ij} = t_{ij} + \delta_{ij}(1 - \sum_{j'=1}^{n} t_{j'i})$, the equations can be expressed in a matrix form: $\boldsymbol{p}(t+1) = T\boldsymbol{p}(t)$. We assume the equilibrium, $\lim_{t\to\infty} \boldsymbol{p}(t)$, to be a unique static state. Accordingly, the eigenvalues of $T$ satisfy $1 = \lambda_0 > \lambda_1 \geqslant \cdots \geqslant \lambda_{n-1} > 0$ [1]. The equilibrium $\boldsymbol{p}(\infty)$ coincides with the zeroth eigenvector of $T$, and the first, second, ... eigenvectors of $T$ represent the slowest relaxation modes.

Metabasins (MBs) in transition probability matrices, are determined similarly with the use of monotonic sequences [2, 3]. A sequence of states $i_1 \to i_2 \to \dots$ is called monotonic if it consists only of most probable transitions. The monotonic sequences with the same terminal state belong to the same MB.

Similarly to the transition rate matrix $K$, the columns and rows of $T$ are rearranged in the MB ordering, $\sigma(1,1), \sigma(1,2), \dots, \sigma(2,1), \sigma(2,2), \dots$, and the resultant matrix is denoted by $T_\sigma$, where $\sigma(\ell, i)$ returns the number $j$ of state $j$ that is the $i$th energy state in MB$_\ell$. Then, we consider the block diagonal matrix $\mathrm{diag}(T_1, \dots, T_\ell, \dots, T_m)$ to be the unperturbed matrix, where $T_\ell$ is given by

$$(T_\ell)_{ij} = t_{\sigma(\ell,i),\sigma(\ell,j)} + \delta_{ij} \sum_{j'=1}^{n_\ell} \left(1 - t_{\sigma(\ell,j'),\sigma(\ell,i)}\right),$$

where $n_\ell$ is the size of MB$_\ell$. Note that $j$th eigenvalues, $\lambda_{\ell,j}$, of $T_\ell$ satisfy $1 = \lambda_{\ell,0} > \lambda_{\ell,1} \geqslant \cdots \geqslant \lambda_{\ell,n_\ell-1} > 0$. To consider the intra-MB relaxation modes, we form $\Lambda_\ell = D_\ell^{-1} T_\ell D_\ell$, with the use of the diagonal matrix $D_\ell = \mathrm{diag}(\sqrt{\boldsymbol{p}_{\ell,0}})$, where $\boldsymbol{p}_{\ell,0}$ is the local equilibrium in MB$_\ell$. It is noteworthy that $\Lambda_\ell$ is the symmetric matrix and can be diagonalized with an orthogonal matrix $S_\ell = \left[\sqrt{\boldsymbol{p}_{\ell,0}}, \boldsymbol{v}_{\ell,1}, \dots, \boldsymbol{v}_{\ell,n_\ell-1}\right]$, where $\boldsymbol{v}_{\ell,j}$ is the $j$th eigenvectors of $\Lambda_\ell$.

To consider the inter-MB transitions, we form the symmetric matrix $\Lambda' = S^T D^{-1} T_\sigma D S$, with $S = \mathrm{diag}(S_1, S_2, \dots)$ and $D = \mathrm{diag}(\sqrt{\boldsymbol{p}_{\mathrm{eq}}})$, where $\boldsymbol{p}_{\mathrm{eq}}$ is the equilibrium of $T_\sigma$. Moreover, to introduce the division of intra-MB relaxation modes into slow and fast modes, we set a certain threshold $\lambda_{\mathrm{cut}}$ satisfying $1 \geqslant \lambda_{\mathrm{cut}} > 0$: the slow relaxation modes are $1 \geqslant \lambda_{\ell,j} \geqslant \lambda_{\mathrm{cut}}$ and the fast relaxation modes are $\lambda_{\mathrm{cut}} > \lambda_{\ell,j} \geqslant 0$. We, then, reorder the columns and lows of $\Lambda'$ in the slow-to-fast relaxation block order, and the resultant matrix is denoted by $\Lambda_{\text{slow-fast}}$. Note that $\Lambda_{\mathrm{slow}}$, defined by the first $n_{\mathrm{slow}} \times n_{\mathrm{slow}}$ submatrix with $n_{\mathrm{slow}}$ denoting the number of unperturbed slow relaxation modes, generally describes an approximate transitions between the slow modes. To obtain the accurate results, we need a renormalized transition matrix $\Lambda^{\mathrm{RG}}_{\mathrm{slow}}$. To this end, we use a Jacobi rotation $\Lambda_{\text{slow-fast}} \mapsto \Lambda^{\mathrm{RG}}_{\text{slow-fast}} = G^T \Lambda_{\text{slow-fast}} G$ such that the resultant couplings between slow and fast modes, $(\Lambda^{\mathrm{RG}}_{\text{slow-fast}})_{ij}$ with $i \leqslant n_{\mathrm{slow}} < j$, are vanishing. Now, the renormalized transition matrix $\Lambda^{\mathrm{RG}}_{\mathrm{slow}}$ is defined by the first $n_{\mathrm{slow}}$-by-$n_{\mathrm{slow}}$ submatrix of $\Lambda^{\mathrm{RG}}_{\text{slow-fast}}$, which reproduces the exact slowest relaxations of the kinetic equation (1).

Table I summarizes the differences between the renormalization procedures for discrete-time and for continuous-time kinetic equations, from which we clearly see that the renormalization procedure for discrete-time kinetic equations is constructed almost in the same way as that for continuous-time kinetic equations developed in the paper.

TABLE I. Differences between discrete-time and continuous-time renormalization procedures: The listed differences are absorbed by the matrix $\Lambda'$ and the definitions of slow modes. In other words, all the procedures after specifying these are exactly the same way between for the discrete-time equation and for the continuous-time equation.

| Time | Matrix to be normalized | $\Lambda'$ | Slow modes |
|---|---|---|---|
| Discrete time | Transition probability matrix $T$ | $S^T D^{-1} T_\sigma D S$ | $1 \geqslant \lambda_{\ell,i} \geqslant \lambda_{\mathrm{cut}}$ |
| Continuous time | Transition rate matrix $K$ | $S^T D^{-1} K_\sigma D S$ | $0 \geqslant \lambda_{\ell,i} \geqslant \lambda_{\mathrm{cut}}$ |

[1] *An Introduction to Markov State Models and Their Application to Long Times cale Molecular Simulation*, edited by G. R. Bowman, V. S. Pande, and F. Noé (Springer, New York, 2013).
[2] For another formularization for MB decompositions of discrete-time Markov state models, see K. Klemm, C. Flamm, and P. F. Stadler, Eur. Phys. J. B 63, 387 (2008).
[3] T. Okushima, T. Niiyama, K. S. Ikeda, and Y. Shimizu, Phys. Rev. E **80**, 036112 (2009).
